# Supplementary material for: Three-body bound states in antiferromagnetic spin ladders
Source: arXiv:2012.01513 ancillary file (2022-09-13)
Supplement: Supplementary file 1 [file supp.pdf]

# Supplemental Material for Accessing Multi-triplons in Spin Ladders using Resonant Inelastic X-ray Scattering

Gary Ferkinghoff<sup>1</sup>, Leanna Müller<sup>1</sup>, Götz S. Uhrig<sup>1</sup>, Umesh Kumar<sup>2</sup>, Benedikt Fauseweh<sup>2</sup>

<sup>1</sup> *Lehrstuhl für Theoretische Physik I, Technische Universität Dortmund, Otto-Hahn-Straße 4, 44221 Dortmund, Germany*

<sup>2</sup> *Theoretical Division, Los Alamos National Laboratory, Los Alamos, New Mexico 87545, USA*

## S1: Triplon representation

In this paper, the Hamiltonian

$$H = J_{\text{rung}} \sum_i \mathbf{S}_{i,1} \mathbf{S}_{i,2} + J_{\text{leg}} \sum_{i,\tau} \mathbf{S}_{i,\tau} \mathbf{S}_{i+1,\tau} \quad (1)$$

and the observables

$$O^I = S_{i,\tau}^z \quad (2a)$$

$$O^{\text{II}} = O_{i,\tau}^{\text{exch}} = \frac{1}{2} \mathbf{S}_{i,\tau} \cdot [J_{\text{leg}}(\mathbf{S}_{i+1,\tau} + \mathbf{S}_{i-1,\tau}) + J_{\text{rung}} \mathbf{S}_{i,\bar{\tau}}] \quad (2b)$$

are investigated. To perform a perturbative expansion using the CUT method for small  $x = J_{\text{leg}}/J_{\text{rung}}$ , we change into second quantization using the triplon framework. A triplon is a quasi-particle describing the excitation of a single dimer. By placing those dimers on the rungs of the ladder, the  $J_{\text{rung}}$  interaction is diagonalized as part of the one-particle triplon energy while  $J_{\text{leg}}$  yields more complex interactions.

For convenience of notation, we will start with a single dimer with basis states  $\{|\uparrow\uparrow\rangle, |\uparrow\downarrow\rangle, |\downarrow\uparrow\rangle, |\downarrow\downarrow\rangle\}$ .

We change to the new triplon basis

$$|s\rangle = |0\rangle = \frac{1}{\sqrt{2}}(|\uparrow\downarrow\rangle - |\downarrow\uparrow\rangle) \quad (3a)$$

$$|x\rangle = (t^x)^\dagger |0\rangle = -\frac{1}{\sqrt{2}}(|\uparrow\uparrow\rangle - |\downarrow\downarrow\rangle) \quad (3b)$$

$$|y\rangle = (t^y)^\dagger |0\rangle = \frac{i}{\sqrt{2}}(|\uparrow\uparrow\rangle + |\downarrow\downarrow\rangle) \quad (3c)$$

$$|z\rangle = (t^z)^\dagger |0\rangle = \frac{1}{\sqrt{2}}(|\uparrow\downarrow\rangle + |\downarrow\uparrow\rangle) \quad (3d)$$

for the singlet and triplet eigenstates, where the triplon operators  $t_\alpha^\dagger$  act on the reference state  $|0\rangle$ .

The triplon operators satisfy the hard-core boson commutation relation

$$\left[ t_i^\alpha, t_j^{\beta\dagger} \right] = \delta_{i,j} \left( \delta_{\alpha,\beta} \left( \mathbb{1} - \sum_{\gamma} t_i^{\gamma\dagger} t_i^{\gamma} \right) - t_i^{\beta\dagger} t_i^{\alpha} \right), \quad (4)$$

where we reintroduced the indices  $i$  for the rung and  $\tau$  for the site on the ladder. Transforming the spin operators

$$2S_{i,1}^\alpha = + t_i^\alpha + t_i^{\alpha\dagger} - i \sum_{\beta\gamma} \epsilon_{\alpha\beta\gamma} t_i^{\beta\dagger} t_i^{\gamma} \quad (5a)$$

$$2S_{i,2}^\alpha = - t_i^\alpha - t_i^{\alpha\dagger} - i \sum_{\beta\gamma} \epsilon_{\alpha\beta\gamma} t_i^{\beta\dagger} t_i^{\gamma} \quad (5b)$$

yields the triplon operator representation of the Hamiltonian

$$\frac{H}{J_{\text{rung}}} = H^{(0)} + H^{(1)} \quad (6)$$

with

$$H^{(0)} = -\frac{3}{4} \sum_i \mathbb{1} + \sum_{i,\alpha} t_i^{\alpha\dagger} t_i^\alpha \quad (7a)$$

$$\begin{aligned} H^{(1)} = & + \frac{x}{2} \sum_{i,\alpha} \left( t_i^{\alpha\dagger} t_{i+1}^\alpha + t_{i+1}^{\alpha\dagger} t_i^\alpha \right) \\ & + \frac{x}{2} \sum_{i,\alpha \neq \beta} t_i^{\alpha\dagger} t_{i+1}^{\beta\dagger} t_i^\beta t_{i+1}^\alpha \\ & - \frac{x}{2} \sum_{i,\alpha \neq \beta} t_i^{\alpha\dagger} t_{i+1}^{\alpha\dagger} t_i^\beta t_{i+1}^\beta \\ & + \frac{x}{2} \sum_{i,\alpha} \left( t_i^{\alpha\dagger} t_{i+1}^{\alpha\dagger} + t_i^\alpha t_{i+1}^\alpha \right) \end{aligned} \quad (7b)$$

and the observables

$$S_{i,\tau}^z = \pm t_i^\alpha + \pm t_i^{\alpha\dagger} - i \sum_{\beta\gamma} \epsilon_{\alpha\beta\gamma} t_i^\beta t_i^\gamma \quad (8a)$$

$$\begin{aligned} O_{i,\tau}^{\text{exch}} = & J_{\text{rung}} \left( -\frac{3}{4} \mathbb{1} + \sum_{\alpha} t_i^{\alpha\dagger} t_i^{\alpha} \right) \\ & + J_{\text{leg}} \sum_{\delta=\pm 1} \left[ \frac{x}{4} \sum_{\alpha} \left( t_i^{\alpha\dagger} t_{i+\delta}^{\alpha} + t_{i+\delta}^{\alpha\dagger} t_i^{\alpha} \right) \right. \\ & + \frac{x}{4} \sum_{\alpha \neq \beta} t_i^{\alpha\dagger} t_{i+\delta}^{\beta\dagger} t_i^{\beta} t_{i+\delta}^{\alpha} \\ & - \frac{x}{4} \sum_{\alpha \neq \beta} t_i^{\alpha\dagger} t_{i+\delta}^{\alpha\dagger} t_i^{\beta} t_{i+\delta}^{\beta} \\ & \left. + \frac{x}{4} \sum_{\alpha} \left( t_i^{\alpha\dagger} t_{i+\delta}^{\alpha\dagger} + t_i^{\alpha} t_{i+\delta}^{\alpha} \right) \right]. \quad (8b) \end{aligned}$$

## S2: Continuous Unitary Transformation

Unitary transformations are often employed to gain an effective Hamiltonian, which preserves the properties of the original Hamiltonian but provides an easier access to the relevant physics. One important strategy is to decouple the particle subspaces such that each particle subspace can be treated separately and single-particle energies as well as  $n$ -particle interactions can easily be identified. Finding such unitary transformations, however, presents a difficult task and developing strategies for systematically generating these transformations pose an even more complicated challenge.

*Continuous unitary transformations (CUTs)* provide a framework to perform these transformations systematically [1]. The CUT method, also known as the *flow equation method* in physics or *double bracket flow* in mathematics, has been introduced in 1994 by Wegner for condensed matter physics [2] and independently by Glazek and Wilson for high-energy physics under the name of *similarity renormalization scheme* [3, 4] and similar flow equations have been studied by the mathematicians Brockett, Chu and Driessel in 1990, called *double bracket flow* [5–7].

As the name suggests, CUTs introduce a continuous transformation

$$H(l) = U(l)H(0)U^\dagger(l) \quad , \quad U^\dagger(l) = U^{-1}(l) \quad (9a)$$

$$H(\infty) = H_{\text{eff}} \quad (9b)$$

with a flow parameter  $l$ . The desired effective Hamiltonian is obtained in the limit of  $l \rightarrow \infty$ . The method becomes systematic by defining the unitary transformation  $U(l)$  by an anti-hermitian generator  $\eta(l)$

$$U(l) = L \exp \left[ \int_0^l \eta(l') dl' \right], \quad \eta^\dagger(l) = -\eta(l) \quad (10)$$

where  $L$  is the  $l$ -ordered product. Inserting (10) in (9b) and derivating with respect to  $l$  yields the flow equation

$$\partial_l H(l) = [\eta(l), H(l)] . \quad (11)$$

By using the notation

$$\hat{H}(l) = \sum_i h_i(l) \hat{A}_i \quad (12a)$$

$$\hat{\eta}(l) = \sum_i \eta_i(l) \hat{A}_i = \sum_i h_i(l) \hat{\eta}[A_i], \quad (12b)$$

where only the coefficients depend on  $l$ , while the operator basis  $\{\hat{A}_i\}$  is constant, the flow equation takes the form

$$\boxed{\partial_l h_i(l) = \sum_{jl} D_{ijl} \eta_j(l) h_l(l)} , \quad (13)$$

where the coefficients  $D_{ijl}$  are obtained by comparing coefficients

$$[\hat{\eta}[A_j], A_l] = \sum_i D_{ijl} A_i . \quad (14)$$

The flow equation (13) can be integrated numerically to obtain the approximated effective Hamiltonian  $H_{\text{eff}} \approx H(l)$  for a sufficiently large  $l$ . The observable  $O_{\text{eff}} \approx O(l) = \sum_i o_i(l) \tilde{A}_i$  can be obtained by simultaneously integrating

$$\boxed{\partial_l o_i(l) = \sum_{jl} \tilde{D}_{ijl} \eta_j(l) o_l(l)} . \quad (15)$$

Thus, the workflow of CUT consists of firstly choosing an appropriate generator, secondly evaluating the commutator found in (13) and thirdly integrating the flow equation.

The generator is usually chosen by a scheme with proven convergence features. For this paper, a variation of the *particle-conserving generator*

$$\hat{\eta}_{\text{pc}}(l) = \sum_{i=0}^{\infty} \sum_{\Delta=1}^{\infty} H_{i,i+\Delta}(l) - H_{i+\Delta,i}(l) \quad (16)$$

has been applied, where  $\tilde{H}_{i,j}$  includes all parts of the Hamiltonian that annihilate  $i$  triplons and create  $j$  triplons. This generator has been suggested by Mielke for banded matrices [8] and independently by Knetter and Uhrig for many-particle systems [9]. This generator scheme attempts to sort all quasiparticle spaces ascending by energy. This can cause problems if the energies of these subspaces overlap during the integration of the flow equation. To deal with this problem, the *particle-sorting generator*

$$\hat{\eta}_{m:n}(l) = \sum_{i=0}^m \sum_{\Delta=1}^{\infty} H_{i,i+\Delta}(l) - H_{i+\Delta,i}(l) \quad (17)$$

has been introduced by Fischer, Duffe and Uhrig [10] and has also been used for this paper. This generator only decouples the subspaces with up to  $m$  particles, while higher subspaces can still be coupled, since terms with more than  $m$  annihilators and their hermitian conjugate counterparts remain in the Hamiltonian.

The *directly evaluated enhanced perturbative CUT (deepCUT)* [11] approach improves the efficiency of the CUT by only considering terms which lead to actual contributions to the searched quantities.

To measure when the CUT has converged, the *residual off-diagonality*

$$\text{ROD} = \sqrt{\sum_i |\eta_i|^2} \quad (18)$$

is employed, which sums the squares of the absolute values of all elements that are to be removed by the CUT. The integration of the flow equation stops when  $\text{ROD} < \text{ROD}_{\min} = 10^{-14} J_{\text{rung}}$  has been reached.

### S3: Lanczos tridiagonalization

To calculate the *dynamic spin structure factor (DSF)* and the *dynamic exchange structure factor (DESF)*

$$S(\mathbf{q}, \omega) = \frac{1}{N} \sum_f \left| \langle f | \sum_{i,\tau} e^{i\mathbf{q}\mathbf{R}_{i,\tau}} S_{i,\tau}^{\alpha} | g \rangle \right|^2 \cdot \delta(E_f - E_g + \omega) \quad (19a)$$

$$S^{\text{exch}}(\mathbf{q}, \omega) = \frac{1}{N} \sum_f \left| \langle f | \sum_{i,\tau} e^{i\mathbf{q}\mathbf{R}_{i,\tau}} O_{i,\tau}^{\text{exch}} | g \rangle \right|^2 \cdot \delta(E_f - E_g + \omega) \quad (19b)$$

a *continued fraction expansion* is applied. We provide the explicit derivation for the DSF, the derivation for the DESF is analogous. The DSF can be calculated as

$$S(\mathbf{q}, \omega) = -\frac{1}{\pi} \text{Im}[G(\mathbf{q}, \omega)] \quad (20)$$

at temperature  $T = 0$  in accordance with the fluctuation-dissipation theorem [12]. The Green function  $G(\mathbf{q}, \omega)$  can be written as a resolvent

$$G(\mathbf{q}, \omega) = \langle g | S_{-q_x, \pm}^{\alpha} \frac{1}{\omega - H(q_x) - E_0 + i0^+} S_{q_x, \pm}^{\alpha} | g \rangle \quad (21)$$

where  $E_0$  denotes the ground state energy and the Fourier transformed spin observable reads

$$S_{q_x, \pm}^{\alpha} = \frac{1}{\sqrt{N}} \sum_i (S_{i,1}^{\alpha} \pm S_{i,2}^{\alpha}) e^{iq_x i}. \quad (22)$$

Note how the cases  $q_y = \{0, \pi\}$  correspond to the sign  $\pm$  in Eq. (22). The Hamiltonian depends on the momentum  $q_x$ . Additionally,  $O_{i,\tau}^{\text{exch}}$  can be handled as a superposition of the two observables  $\mathbf{S}_{i,\tau} \cdot \mathbf{S}_{i+1,\tau}$  and  $\mathbf{S}_{i,\tau} \cdot \mathbf{S}_{i,\bar{\tau}}$ , reducing computational cost. This is especially convenient for  $O_{q_x,-}^{\text{exch}}$ , where the rung coupling  $\mathbf{S}_{i,\tau} \cdot \mathbf{S}_{i,\bar{\tau}}$  disappears.

Using second quantization and the CUT framework, the effective operators and the vacuum state are used to yield the Green function

$$G(\mathbf{q}, \omega) = \langle 0 | S_{-q_x, \pm, \text{eff}}^{\alpha} \frac{1}{\omega - H_{\text{eff}}(q_x) - E_0 + i0^+} S_{q_x, \pm, \text{eff}}^{\alpha} | 0 \rangle. \quad (23)$$

By tridiagonalizing

$$H_{\text{eff}}(q_x) = \begin{pmatrix} a_0 & b_0 & 0 & \cdots \\ b_0 & a_1 & b_1 & \cdots \\ 0 & b_1 & a_2 & \cdots \\ \vdots & \vdots & \vdots & \ddots \end{pmatrix} \quad (24)$$

with respect to the state  $S_{q_x, \pm, \text{eff}}^{\alpha} | 0 \rangle$ , we can perform the continued fraction expansion [13, 14]

$$G(\mathbf{q}, \omega) = \frac{b_0^2(\mathbf{q})}{\omega - a_0(\mathbf{q}) - \frac{b_1^2(\mathbf{q})}{\omega - a_1(\mathbf{q}) - \dots}}. \quad (25)$$

The tridiagonalized form (24) is calculated using the *Lanczos algorithm*, which calculates an orthogonal basis

$$|\Psi_0\rangle = S_{q_x, \pm, \text{eff}}^{\alpha} | 0 \rangle \quad (26a)$$

$$|\Psi_1\rangle = (H_{\text{eff}} - a_0) |\bar{\Psi}_0\rangle \quad (26b)$$

$$|\Psi_{n+1}\rangle = (H_{\text{eff}} - a_n) |\bar{\Psi}_n\rangle - b_n^2 |\bar{\Psi}_{n-1}\rangle \quad \forall n \in \mathbb{N}_+ \quad (26c)$$

$$|\bar{\Psi}_n\rangle = \frac{|\Psi_n\rangle}{b_n} \quad \forall n \in \mathbb{N}_0 \quad (26d)$$

with the *Lanczos coefficients (LC)*

$$a_n(\mathbf{q}) = \frac{\langle \Psi_n | H_{\text{eff}}(q_x) | \Psi_n \rangle}{\langle \Psi_n | \Psi_n \rangle} \quad \forall n \in \mathbb{N}_0 \quad (27a)$$

$$b_0^2(\mathbf{q}) = \langle \Psi_0 | \Psi_0 \rangle \quad (27b)$$

$$b_n^2(\mathbf{q}) = \frac{\langle \Psi_n | \Psi_n \rangle}{\langle \Psi_{n-1} | \Psi_{n-1} \rangle} \quad \forall n \in \mathbb{N}_+ . \quad (27c)$$

To calculate how the operators work on the states, the  $n$ -particle states  $|r_0, \alpha_0\rangle \dots |r_n, \alpha_n\rangle$  with triplons of flavors  $\alpha_i$  at rungs  $r_i$  (with  $r_{i+1} > r_i \forall i$ ) can be Fourier transformed to

$$|q_x, \alpha_0\rangle = \frac{1}{\sqrt{N}} \sum_{r_0} e^{iq_x r_0} |r_0, \alpha_0\rangle \quad (28a)$$

$$|q_x, \alpha_0\rangle |r_1, \alpha_1\rangle = \frac{1}{\sqrt{N}} \sum_{r_0} e^{iq_x \frac{r_0+r_1}{2}} |r_0, \alpha_0\rangle |r_1, \alpha_1\rangle \quad (28b)$$

$$|q_x, \alpha_0\rangle \dots |r_n, \alpha_n\rangle = \frac{1}{\sqrt{N}} \sum_{r_0} e^{iq_x \frac{r_0+\dots+r_n}{n+1}} |r_0, \alpha_0\rangle \dots |r_n, \alpha_n\rangle . \quad (28c)$$

If  $|b_n| < 10^{-8}$  at any point, we assume that the Krylov subspace has been traversed fully and terminate the algorithm. However, since the basis of possible multi-particle states is infinite, we introduce a maximum distance  $d_{\text{max}}$  between the particles, so that only states with

$$r_{i+1} \in \{r_i + 1, r_i + 2, \dots, r_i + d_{\text{max}}\} \quad (29)$$

are considered. Before performing the Lanczos tridiagonalization,  $|\Psi_0\rangle$  and  $H_{\text{eff}}$  are converted to a sparse matrix representation. In this way,  $H_{\text{eff}}|\beta_i\rangle$  must only be calculated once for each basis state  $|\beta_i\rangle$ . The basis only includes states that can be created by applying  $H_{\text{eff}}$  repeatedly on  $|\Psi_0\rangle$  and which fulfill (29).

The Lanczos tridiagonalization was performed for 201 different values of  $q_x$ . So we only apply  $H_{\text{eff}}$  to each  $|\beta_i\rangle$  once, the matrix representation is calculated for a general  $q_x$  by explicitly storing the exponents of the phase factors that arise during the calculation. For each  $q_x$ , the operator was then transformed into a sparse matrix of complex doubles. This approach showed a significant reduction of computation time for calculations up to 3-quasiparticle space. Only for 4-quasiparticle calculations, where memory consumption proved to be the greater issue, the general  $Q$ -representation was omitted and the explicit matrices were calculated anew each time.

Because of the  $d_{\text{max}}$ -condition (29) and the resulting reduction of the basis, some states can only be represented approximately. For the two-leg ladder, the order of the CUT and the number of

sites that can be hopped by an excitation per application of  $H_{\text{eff}}$  coincide. Therefore the LC will be affected by the truncation for

$$n > \frac{d_{\text{max}}}{\text{CUT-order}} . \quad (30)$$

Nevertheless, most coefficients after this point can still be used without detrimental effect. As long as  $d_{\text{max}}$  is chosen large enough, the LC  $a_n$  and  $b_n$  converge to a limiting value  $a_\infty$  (or  $b_\infty$ ), possibly with slight oscillation around the limiting values. For even larger  $n$  the LC become unstable again and are truncated. The truncation point  $n_{\text{LC}}$  has been determined for each calculation by hand. The convergence values  $a_\infty$  and  $b_\infty$  were determined by averaging over the last few LC.

A *Square-root terminator*  $G_\infty$  [13, 14] is used to increase the accuracy of the continued fraction expansion (25)

$$G(\mathbf{q}, \omega) = \frac{b_0^2(\mathbf{q})}{\omega - a_0(\mathbf{q}) - \frac{b_1^2(\mathbf{q})}{\dots - G_\infty(\mathbf{q}, \omega)}} . \quad (31)$$

Without writing out the dependencies on  $\mathbf{q}$  and  $\omega$  explicitly, the definition

$$G_\infty := \frac{b_\infty^2}{\omega - a_\infty - G_\infty} \quad (32)$$

leads to

$$G_\infty = \begin{cases} \frac{\omega - a_\infty}{2} - \sqrt{\left(\frac{\omega - a_\infty}{2}\right)^2 - b_\infty^2} & , \omega > E_u \\ \frac{\omega - a_\infty}{2} - i\sqrt{b_\infty^2 - \left(\frac{\omega - a_\infty}{2}\right)^2} & , \omega \in [E_l, E_u] \\ \frac{\omega - a_\infty}{2} + \sqrt{\left(\frac{\omega - a_\infty}{2}\right)^2 - b_\infty^2} & , \omega < E_l \end{cases} \quad (33)$$

with the upper and lower edge band of the continuum

$$E_u = a_\infty + 2b_\infty , \quad (34)$$

$$E_l = a_\infty - 2b_\infty . \quad (35)$$

These approximations of the upper and lower edge, which depend on the accuracy of the Lanczos coefficients, are also used for the continuum edges in the plots.

This approach works well for calculating  $\text{Im}[G(\mathbf{q}, \omega)]$ , which is needed for the DSF or DESF in (20). However, outside of the continuum, the (anti-)bound states are calculated by diagonalizing (24). For all eigenvalues  $\epsilon \notin [E_l, E_u]$  outside of the continuum with eigenvector  $|\epsilon\rangle$  the corresponding weight is calculated by

$$I_\epsilon = \langle \epsilon | \Psi_0 \rangle . \quad (36)$$

For the single-particle subspace, where no continuum exists, the weight is given by  $I_\epsilon = \langle \Psi_0 | \Psi_0 \rangle$  and no Lanczos iteration is necessary.

For the plots, the spectral weights of the bound states is depicted by using a Lorentzian broadening

$$G_{\text{Lorentz}}(\omega, \epsilon) = -i \frac{I_\epsilon \gamma}{(\omega - \epsilon)^2 + \gamma^2} \quad (37)$$

with  $\gamma = 0.05$ . This broadening allows for good comparison between the continuum spectral weight and the weight in the bound states. A similar broadening for contributions inside of the continuum can be applied through substituting  $\omega \rightarrow \omega + i\delta$  in (31), but this has not been done for the plots presented here. Note that for experimental purposes, a Gaussian broadening due to measuring inaccuracies might be the relevant broadening effect. Here, however, we choose a Lorentzian broadening for computational convenience.

#### S4: Non-spin-conserving RIXS response

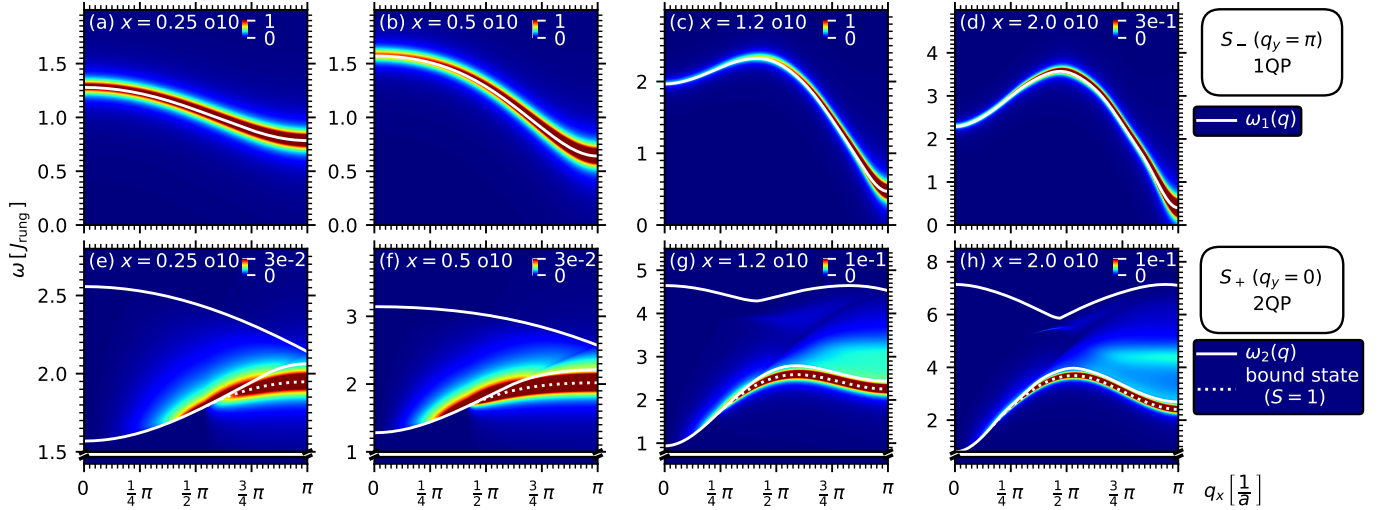

FIG. 1: DSF results for the observables for  $q_y = \pi$  (a-d) and for  $q_y = 0$  (e-h).

The dominant contribution in the NSC channel comes from the DSF. We show in Fig. 1 the DSF as function of momentum  $\mathbf{q} = (q_x, q_y)$  and energy  $\omega$  for different values of the coupling  $x$ .

In the strong rung coupling regime the  $q_y = \pi$  response is dominated by the single triplon contribution, see Fig. 1(a)-(d). As the leg coupling is increased the triplons become more dispersive and the bandwidth increases. The next leading contribution for the DSF for  $q_y = \pi$  comes from

the three-triplon sector. For the parameter regime we are investigating the three-triplon sector has a negligible spectral weight, however its effect can still be seen in the dip of the single triplon dispersion for  $x > 0.5$ , i.e., the lower three-triplon boundary is pushing down the single-triplon dispersion at  $q_x = 0$  due to level repulsion. This leads to a shift in the position of the dispersion maximum from  $q_x = 0$  to  $q_x = \pi/2$ . At the same time this is also a precursor of spin chain physics: in the limit  $J_{\text{rung}} \rightarrow 0$  the dispersion is symmetric at  $q_x = \pi/2$  with gap closing at  $q_x = 0$  and  $q_x = \pi$ .

In contrast, the contribution for  $q_y = 0$  has even parity. The single-triplon contribution vanishes exactly and the leading contribution comes from the two-triplon sector, see Fig. 1(e)-(h). In the NSC channel, we can clearly identify the  $S = 1$  bound state. It holds a significant portion of the overall spectral weight until it merges with the two-triplon continuum. The continuum itself is rather featureless.

## S5: Numerical details

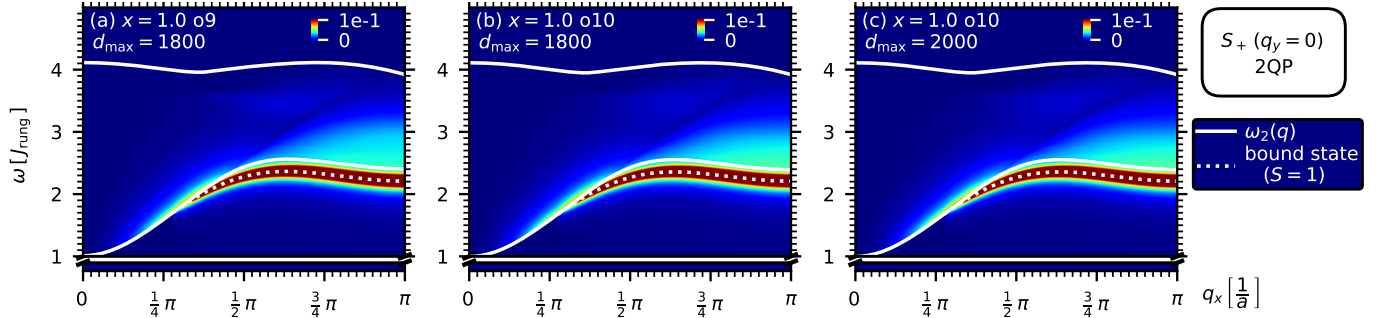

FIG. 2: Exemplary comparison of the 2-triplon DSF shown in the main paper (right), DSF calculated with lowered  $d_{\text{max}}$  (middle) and DSF calculated with lowered CUT order (left).

The parameters for all presented DSF and DESF results are listed in table I. The discretization in  $\omega$  is set to 2000 points for all plots.  $n_{\text{QP}}$  is the considered multi-particle subspace,  $x = J_{\text{leg}}/J_{\text{rung}}$  the perturbation parameter, order the perturbation order in the CUT,  $n_{\text{LC}}$  the number of considered Lanczos coefficients and  $n_{q_x}$  the discretization in  $q_x$  for the plots.

While the main paper only shows the DESF results, Fig. 1 depicts the DSF for 1- and 2-triplon space. The main features agree well with the results in [15], but offers a higher resolution without any finite-size effects.

To check how well the data has converged, we compare individual plots with their counterpart with

| Channel              | $\hat{O}$           | $q_y$ | $n_{\text{QP}}$ | $\hat{\eta}$ | $x$  | order  | $d_{\text{max}}$ | $n_{\text{LC}}$ | $n_{q_x}$ |
|----------------------|---------------------|-------|-----------------|--------------|------|--------|------------------|-----------------|-----------|
| NSC                  | $S_-$               | $\pi$ | 1               | 1:n          | 0.25 | o10    | -                | 1               | 201       |
|                      |                     |       |                 |              | 0.5  | o10    | -                | 1               | 201       |
|                      |                     |       |                 |              | 1.2  | o10    | -                | 1               | 201       |
|                      |                     |       |                 |              | 2.0  | o10    | -                | 1               | 201       |
| (Fig 1 a-d)          |                     |       |                 |              |      |        |                  |                 |           |
| NSC                  | $S_+$               | 0     | 2               | 2:n          | 0.25 | o10    | 2000             | 1000            | 201       |
|                      |                     |       |                 |              | 0.5  | o10    | 2000             | 800             | 201       |
|                      |                     |       |                 |              | 1.2  | o10    | 2000             | 600             | 201       |
|                      |                     |       |                 |              | 2.0  | o10    | 2000             | 500             | 201       |
| (Fig 1 e-h)          |                     |       |                 |              |      |        |                  |                 |           |
| SC                   | $O_+^{\text{exch}}$ | 0     | 2               | 2:n          | 0.25 | o10    | 2000             | 1000            | 201       |
|                      |                     |       |                 |              | 0.5  | o10    | 2000             | 900             | 201       |
|                      |                     |       |                 |              | 1.2  | o10    | 2000             | 600             | 201       |
|                      |                     |       |                 |              | 2.0  | o10    | 2000             | 500             | 201       |
| (Main paper, Fig. 1) |                     |       |                 |              |      |        |                  |                 |           |
| SC                   | $O_-^{\text{exch}}$ | $\pi$ | 3               | 3:n+2:n      | 0.25 | o9+o10 | 1000             | 560             | 201       |
|                      |                     |       |                 |              | 0.5  | o8+o10 | 1000             | 600             | 201       |
|                      |                     |       |                 |              | 1.2  | o6+o10 | 1000             | 500             | 201       |
|                      |                     |       |                 |              | 2.0  | o5+o10 | 1000             | 500             | 201       |
| (Mixed approach)     |                     |       |                 |              |      |        |                  |                 |           |
| (Main paper, Fig. 2) |                     |       |                 |              |      |        |                  |                 |           |
| NSC                  | $S_+$               | 0     | 2               | 2:n          | 1.0  | o9     | 1800             | 900             | 201       |
|                      |                     |       |                 |              | 1.0  | o10    | 1800             | 900             | 201       |
| (Fig. 2)             |                     |       |                 |              |      |        |                  |                 |           |
| SC                   | $O_+^{\text{exch}}$ | 0     | 2               | 2:n          | 1.0  | o10    | 2000             | 600             | 201       |
| SC                   | $O_-^{\text{exch}}$ | $\pi$ | 3               | 3:n          | 1.0  | o6     | 1000             | 500             | 201       |
| (Fig. 4)             |                     |       |                 |              |      |        |                  |                 |           |
| SC                   | $O_+^{\text{exch}}$ | 0     | 2,4             | 2:n          | 0.25 | o10    | 60               | 30              | 51        |
|                      |                     |       |                 |              | 0.5  | o10    | 60               | 30              | 51        |
|                      |                     |       |                 |              | 1.2  | o10    | 80               | 30              | 51        |
|                      |                     |       |                 |              | 2.0  | o10    | 60               | 30              | 51        |
| (Fig. 6)             |                     |       |                 |              |      |        |                  |                 |           |

TABLE I: Technical parameters of all plots.

a lower number of Lanczos coefficients due to a lower  $d_{\text{max}}$  in the continued fraction expansion and with their counterpart with a lower perturbation order in the CUT in Fig. 2 for  $x = 1.0$ . It

shows no significant differences. Similar comparisons for the DESF and other parameters display a similar level of convergence.

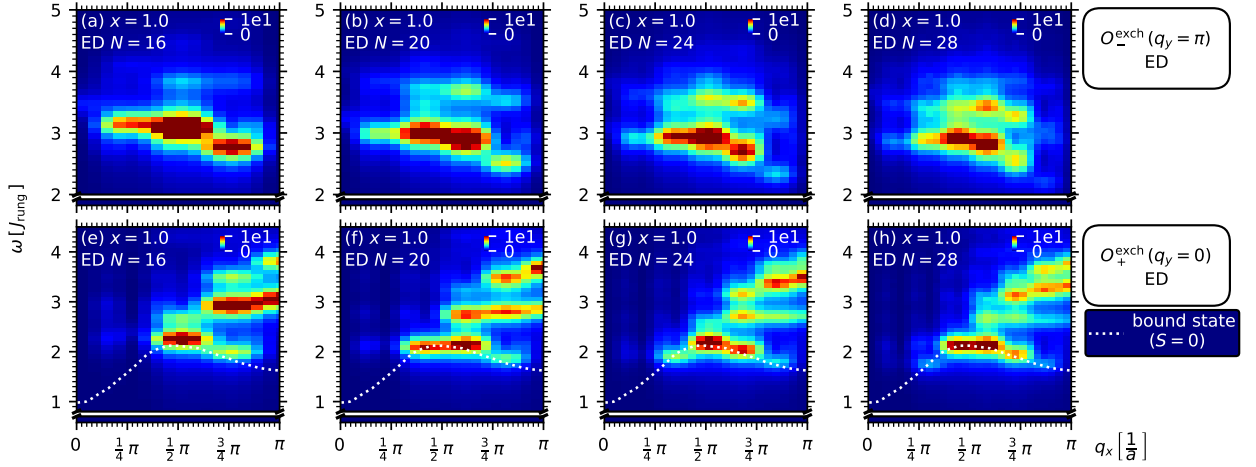

FIG. 3: DESF for  $q_y = \pi$  (a-d) and  $q_y = 0$  (e-h) calculated with exact diagonalization for different numbers of sites  $N$ .

### A. Comparison with Exact diagonalization

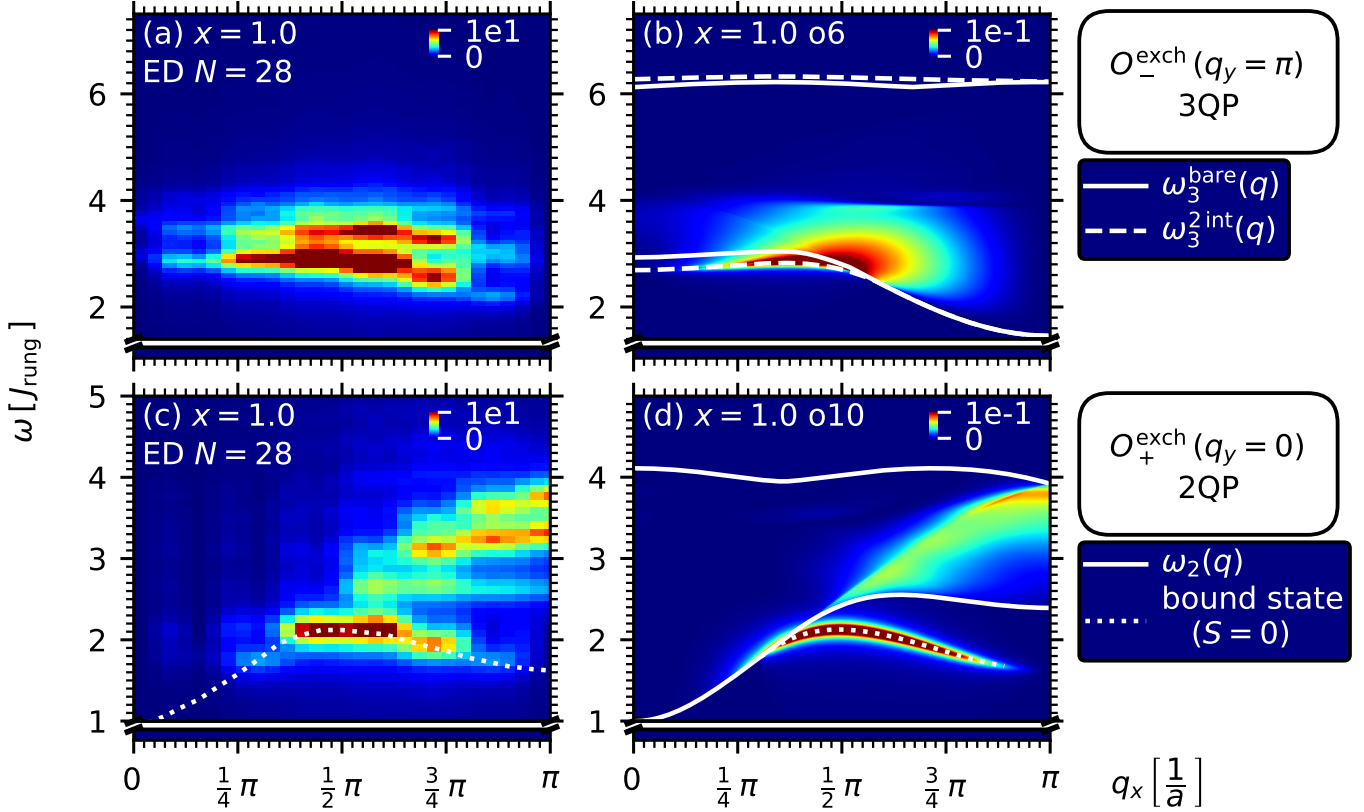

FIG. 4: Exemplary comparison of the 2-triplon DESF calculated with exact diagonalization (left) and the CUT approach shown in the main paper (right).

Figure 4 shows a comparison of the DESF at  $x = 1.0$  with results obtained through *exact diagonalization* (ED). The main features can be seen with both methods, but the CUT results provide an exceedingly higher resolution without finite-size artifacts. In contrast the ED results show strong finite-size artifacts, as can be seen for instance in Fig. 3, where we can see features disappearing and reappearing for  $q_y = 0$  when the number of sites  $N$  is increased. In conclusion the ED results confirm the CUT calculations and verify our approach.

### B. 4-Triplon results

In the main paper, the leading 2-triplon order of the DESF for  $q_y = 0$  in the *spin-conserving* (SC) *channel* has been shown. Further calculations for the 4-triplon subspace have been performed as well. Due to numerical limitations and the problem of unstable flow equations at higher orders,

the 2:n-generator is used and only 51 different values of  $q_x$  and around 30 Lanczos coefficients could be calculated and are shown in Fig. 6. The detailed parameters can be found in Tab. I.

While the results are very coarse due to the low number of LCs, we can still make qualitative statements. The combined DESF for 2-triplons and 4-triplons shows that the spectral weight of the 4-triplon subspace is negligibly small. However, the subspaces do overlap for  $x \geq 0.5$  and some of the main features of 4-triplon space are in the region of 2-triplon space. Further 4-triplon features can be seen for higher energies around  $q_x = 0$ .

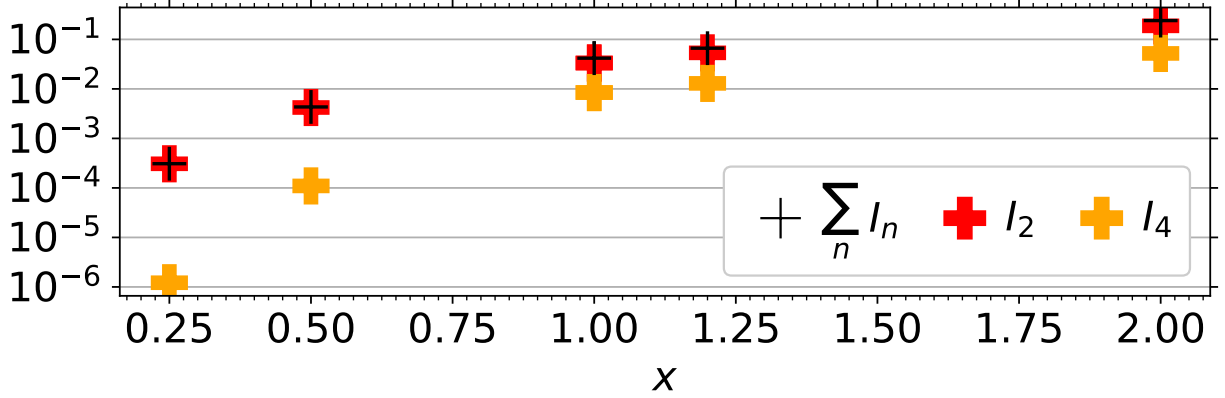

FIG. 5: Spectral weight of the DESF in two-triplon subspace ( $I_2$ ), four-triplon subspace ( $I_4$ ), and all subspaces ( $\sum_n I_n$ ) calculated for  $x \in \{0.25, 0.5, 1.0, 1.2, 2.0\}$  by integrating over  $b_0^2(q_x)$ , see (38).

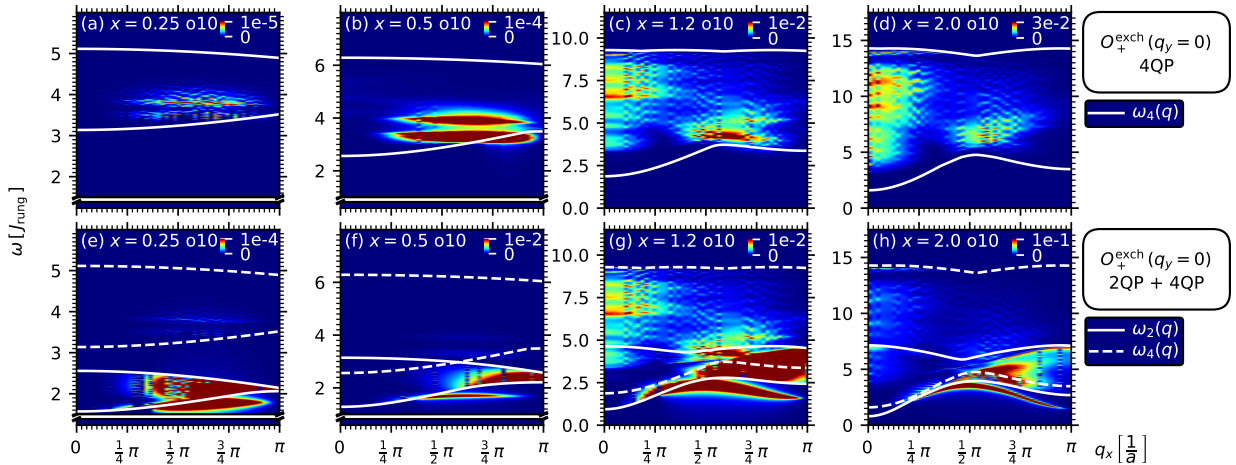

FIG. 6: Results for the DESF in 4-triplon space (a-d) and combined results of 2-triplon space and 4-triplon space (e-h), all calculated with  $n_{\text{LC}} = 30$  Lanczos coefficients.

Additionally the full spectral weights

$$I = \frac{1}{\pi} \int_0^\pi b_0^2(q_x) dq_x \quad (38)$$

for two-triplon subspace and four-triplon subspace are shown in Fig. 5. We can see that while the relative weight of four-triplon space increases with  $x$ , it still lies one order of magnitude below the two-triplon weight. Furthermore the area over which the spectral weight is spread is significantly larger for four-triplons than for two-triplons, as can be seen in Fig. 6 (d) and (h). This leads to the conclusion that the four-triplon DESF does not interfere with the two-triplon DESF in a significant way for  $x \lesssim 2$ .

- 
- [1] S. Kehrein, *The Flow Equation Approach to Many-Particle Systems*, 217th ed. (Springer Tracts in Modern Physics, Springer-Verlag Berlin Heidelberg, 2006).
  - [2] F. Wegner, *Ann. der Phys.* **3**, 77 (1994).
  - [3] S. D. Glazek and K. G. Wilson, *Phys. Rev. D* **48**, 5863 (1993).
  - [4] S. D. Glazek and K. G. Wilson, *Phys. Rev. D* **49**, 4214 (1994).
  - [5] M. T. Chu and K. R. Driessel, *SIAM J. Numer. Anal.* **27**, 1050 (1990).
  - [6] R. W. Brockett, *Lin. Alg. and its Appl.* **146**, 79 (1991).
  - [7] M. T. Chu, *Fields Institute Communications* **3**, 87 (1994).
  - [8] A. Mielke, *Europ. Phys. Jour. B* **5**, 605 (1998).
  - [9] C. Knetter and G. S. Uhrig, *Europ. Phys. Jour. B* **13**, 209 (2000).
  - [10] T. Fischer, S. Duffe, and G. S. Uhrig, *New. Jour. of Phys.* **12**, 033048 (2010).
  - [11] H. Krull, N. A. Drescher, and G. S. Uhrig, *Phys. Rev. B* **86**, 125113 (2012).
  - [12] D. Chandler, *Introduction to Modern Statistical Mechanics* (Oxford University Press, 1987).
  - [13] D. G. Pettifor and D. L. Weaire, *The Recursion Method and its Applications*, 58th ed. (Springer Verlag, Berlin, 1985).
  - [14] V. S. Viswanath and G. Müller, *The Recursion Method* (Springer Verlag, Berlin, 1994).
  - [15] U. Kumar, A. Nocera, E. Dagotto, and S. Johnston, *Phys. Rev. B* **99**, 205130 (2019).
